# Supplementary material for: Understanding the Properties of Generated Corpora
Source: arXiv:2206.11219 source file (2022-10-27)
Supplement: Supplementary file 1 [file appendix.tex]

\newcommand{\tablebox}[1] {
  \noindent\fbox{%
    \parbox{\textwidth}{\ttfamily #1
      }}}
      
\onecolumn
\section*{Appendix}

%%%%%%%%%%%%%%%%%%%%%%%%%%%%%%%%%%%%%%%%%%%%%%%%%%%%%%%%%%%%%
%%%%%%%%%%%%%%%%%%%%%%%%%%%%%%%%%%%%%%%%%%%%%%%%%%%%%%%%%%%%%
%%%%%%%%%%%%%%%%%%%%%%%%%%%%%%%%%%%%%%%%%%%%%%%%%%%%%%%%%%%%%

\begin{figure}[h!]
\centering
\begin{subfigure}{1\textwidth}
  \centering
  \tablebox{
  \begin{itemize}[noitemsep]
      \item Trump s EPA Chief I Do nt Think He s
      \item Trump s Latest Travel Ban On Climate Change
      \item  Trump s Budget Cuts To Fund Obamacare
      \item The US Military Policy Is A Disaster
      \item Trump s Budget Cuts To Ban On His Own Media
  \end{itemize}
  }
  \caption{VAE}
\end{subfigure}
\begin{subfigure}{1\textwidth}
  \centering
  \tablebox{
  \begin{itemize}[noitemsep]
    \item Senate Republicans Vote On Bringing Back Trump
    \item Trump And Clinton And Sanders Supporters
    \item GOP Senator Donald Trump Should Be Known For Climate Change
    \item Trump Picks Up On North Korea NATO In Ohio
    \item Read The Full Text Of The GOP Convention Is Going To Be A Mess And Transparency
    \end{itemize}
 }
  \caption{CVAE}
  \end{subfigure}
  \begin{subfigure}{1\textwidth}
 \tablebox{
 \begin{itemize}[noitemsep]
    \item Progressives Plan Day Of Demonstrations In St. Louis Police Officer Involved In Killing Of Muslim Women 
    \item How US Policy or a Tar Baby He Ca n't See A Social Security
    \item N.J. Senate Passes Zika Bill That Could Mean .
    \item Bobby Jindal Uncomfortable With Donald Trump Says He No Longer \item A National Museum For Black Communities
    Baltimore Mayor Stephanie Rawlings - Blake Will Not Face Corruption Charges.
    \end{itemize}
    }%
  \caption{MM}
  \end{subfigure}
  \begin{subfigure}{1\textwidth}
  \tablebox{
  \begin{itemize}[noitemsep]
    \item Did President Obama 's Butt Steve King Are Throwing Except For \item Bill Clinton ? Well , As You Can See , They Can not Be Put Out .
    \item Wendy Short Embraces Her On Twitter But Has Enough Votes To Run
    \item Marco Rubio Says He Should n't Support Republicans Signing ' \item Obamacare ' Repeal Bill
    \item What About China ? In What Is , Anyway , Russia Conspiracy ?
    Trump Risks Embarrassing GOP Over His Trade Deal With Indiana
     \end{itemize}
}
 \caption{GPT-2}
\end{subfigure}
\begin{subfigure}{1\textwidth}
  \centering
  \tablebox{
  \begin{itemize}[noitemsep]
    \item huffpost rise what february need to know on you
    \item waiting forever to balloting this website wants to hand you free pizza
    \item trump exercises less communications communication theory control than nixon
    \item look the first same sex weddi
    \item trey gowdy plays down report that congressman will leave congress
    \end{itemize}
 }
  \caption{EDA}
\end{subfigure}
 \caption{Sample sentence by the different models when trained on the News  dataset}
 \label{figsamples_news}
\end{figure}

%%%%%%%%%%%%%%%%%%%%%%%%%%%%%%%%%%%%%%%%%%%%%%%%%%%%%%%%%%%%%
%%%%%%%%%%%%%%%%%%%%%%%%%%%%%%%%%%%%%%%%%%%%%%%%%%%%%%%%%%%%%
%%%%%%%%%%%%%%%%%%%%%%%%%%%%%%%%%%%%%%%%%%%%%%%%%%%%%%%%%%%%%

\begin{figure}[h!]
\centering
\begin{subfigure}{1\textwidth}
  \centering
  \tablebox{
  \begin{itemize}[noitemsep]
    \item I like this phone but I have nt had any problems with it
    \item excelente producto llego con el tiempo de I RECOMMEND
    \item great product and fast shipping great deal
    \item Did not work well Battery life is poor
    \item I like the phone Very good
    \end{itemize}
  }
  \caption{VAE}
\end{subfigure}
\begin{subfigure}{1\textwidth}
  \centering
  \tablebox{
  \begin{itemize}[noitemsep]
    \item I love this phone a great
    \item Very good phone works perfectly in Venezuela
    \item very good I like this product
    \item Works perfect with Africa
    \item It was good and it was not
    \end{itemize}
 }
  \caption{CVAE}
  \end{subfigure}
  \begin{subfigure}{1\textwidth}
 \tablebox{
 \begin{itemize}[noitemsep]
    \item Loving my new 5s
    \item Awesome cellphone , much better than the 5s and it looked like someone threw it in Argentina
    \item I love this phone for my mom loves her new phone so much ! ! !
    \item i recieved it in excellent condition , works with TracFone .
    \item phone will not come with a battery .
    \end{itemize}
    }%
  \caption{MM}
  \end{subfigure}
  \begin{subfigure}{1\textwidth}
  \tablebox{
  \begin{itemize}[noitemsep]
    \item Nice little phone .. price was right.ok
    \item Great smart phone - capable of standing up to an all day army .
   \item Phone did not work so caught the signal too much .
    \item It did my thing when the phone was advertised.works just fine now
    \item A productive phone but the battery dies really fast .
    \end{itemize}
}
 \caption{GPT-2}
\end{subfigure}
\begin{subfigure}{1\textwidth}
  \centering
  \tablebox{
  \begin{itemize}[noitemsep]
    \item shipped quickly outstanding quality works just fine
    \item great phone and very only thing is camara touchsensitive
    \item works great outstanding lots of space to get apps
    \item this is not a good typesetters case it has not stay on
    \item so far so interahamwe good works well
    \end{itemize}
 }
  \caption{EDA}
\end{subfigure}
 \caption{Sample sentence by the different models when trained on the Amazon  dataset}
 \label{figsamples_news}
\end{figure}

%%%%%%%%%%%%%%%%%%%%%%%%%%%%%%%%%%%%%%%%%%%%%%%%%%%%%%%%%%%%%
%%%%%%%%%%%%%%%%%%%%%%%%%%%%%%%%%%%%%%%%%%%%%%%%%%%%%%%%%%%%%
%%%%%%%%%%%%%%%%%%%%%%%%%%%%%%%%%%%%%%%%%%%%%%%%%%%%%%%%%%%%%

\begin{figure}[h!]
\centering
\begin{subfigure}{1\textwidth}
  \centering
  \tablebox{
  \begin{itemize}[noitemsep]
    \item What are the side effects of taking a bad breath
    \item what is the difference between a viral and a steam practice
    \item What are the side effects of taking a heart
    \item how can I cure my teeth
    \item What is the difference between a coma and a general

    \end{itemize}
  }
  \caption{VAE}
\end{subfigure}
\begin{subfigure}{1\textwidth}
  \centering
  \tablebox{
  \begin{itemize}[noitemsep]
    \item How can you make your teeth come
    \item why does my vagina stink when I eat
    \item how can u get rid of pain
    \item How do you stop you eyes from the bad effects
    \item what are the effects of taking intercourse

    \end{itemize}
 }
  \caption{CVAE}
  \end{subfigure}
  \begin{subfigure}{1\textwidth}
 \tablebox{
 \begin{itemize}[noitemsep]
    \item I occasionally get nauseated after sex , any ideas for a canker sore ?
    \item How do you stop a pimple and a periodontist and an endoscopy ?
    \item How can I lose more fat exercising in the body at repairing ?
    \item What effect does PMS have on her fingers swell up can figure out that is used eg blood , sperm , etc.?
    \item what i wana do with being obese ?

    \end{itemize}
    }%
  \caption{MM}
  \end{subfigure}
  \begin{subfigure}{1\textwidth}
  \tablebox{
  \begin{itemize}[noitemsep]
    \item playful questions internally , what are the goings on with sleep ?
    \item What is the root cause of severe Dysfunction ?
    \item what the purpose of an appendix is ?
    \item how can i prevent myself from getting colds in the morning ?
    \item What has been done to remove fungal teeth in a dentures ?

    \end{itemize}
}
 \caption{GPT-2}
\end{subfigure}
\begin{subfigure}{1\textwidth}
  \centering
  \tablebox{
  \begin{itemize}[noitemsep]
    \item one why do i get heart palpitations
    \item how do person you convince someone to stop smoking
    \item how do you find a bash good psychotherapist
    \item why is life story so horrible
    \item how does decrease effective ways to the your weight

    \end{itemize}
 }
  \caption{EDA}
\end{subfigure}
 \caption{Sample sentence by the different models when trained on the Yahoo dataset}
 \label{figsamples_news}
\end{figure}
